# Supplementary material for: Kronecker states: a powerful source of multipartite maximally entangled states in quantum information
Source: arXiv:2504.16256 source file (2025-04-22)
Supplement: Supplementary file 1 [file Appendix00.tex]

In this appendix we show a procedure to obtain the irreducible representations of $S_n$  by using the Schur-Weyl duality instead of the Yamanouchi algorithm. Consider for example $S_3$ and the irrep $[1]$. If we want to compute the matrix representation of some permutation, for example $(23)$, first write the action in the computational basis
\begin{equation}
    (23)= \left( \begin{array}{cccccccc}
     1    & & & & & & & \\
       & & 1& & & & & \\
          &1 & & & & & &\\
              & & & 1& & & &\\
                 & & & &1 & & &\\
                     & & & & & &1 &\\
                         & & & & & 1& &\\
                             & & & & & & &1
    \end{array}\right)
\end{equation}
which can be seen easier as 
\begin{equation}
\begin{gathered}
   (23)=\ket{000}\bra{000}+\ket{001}\bra{010}+\ket{010}\bra{001}+\ket{011}\bra{011} \\
 +  \ket{100}\bra{100}+\ket{101}\bra{110}+\ket{110}\bra{101}+\ket{111}\bra{111} .
\end{gathered}
\end{equation}
We want to compute the matrix elements that corresponds to 
\begin{equation}
  D^{[1]}(23)_{ij}=  \bra{1,Y_i}(23)\ket{1,Y_j}
\end{equation}
We already know how to compute this elements when appending some weight $\omega$, but from Schur-Weyl duality it is known that the different $\omega$ values only correspond to different multiplicities of the representation, so, by picking some $\omega (i,e,. \omega=1)$
\begin{equation}
\begin{gathered}
    D^{[1]}(23)_{ij}=  \bra{1,1,Y_i}(23)\ket{1,1,Y_j}\\
    =\bra{1,1,Y_i}\left(\ket{000}\bra{000}+\ket{001}\bra{010}+\ket{010}\bra{001}+\ket{011}\bra{011} \right.\\
 \left.  \ket{100}\bra{100}+\ket{101}\bra{110}+\ket{110}\bra{101}+\ket{111}\bra{111} \right)\ket{1,1,Y_j}\\
 =\bra{1,1,Y_i}\left(\ket{001}\bra{010}+\ket{010}\bra{001}+ \ket{100}\bra{100} \right)\ket{1,1,Y_j}
\end{gathered}
\end{equation}
Now lets compute the four elements
\begin{equation}
    \begin{gathered}
     D^{[1]}(23)_{11}=\bra{1,1,\{0,0,1\}}\ket{001}\bra{010}\ket{1,1,\{0,0,1\}}+\bra{1,1,\{0,0,1\}}\ket{010}\bra{001}\ket{1,1,\{0,0,1\}}\\+ \bra{1,1,\{0,0,1\}}\ket{100}\bra{100} \ket{1,1,\{0,0,1\}}\\
     =\sqrt{\frac{2}{3}}\left(-\sqrt{\frac{1}{6}}\right)+\left(-\sqrt{\frac{1}{6}}\right)\left(\sqrt{\frac{2}{3}}\right)+\left(-\sqrt{\frac{1}{6}}\right)\left(-\sqrt{\frac{1}{6}}\right)=-\frac{1}{2}\\
     D^{[1]}(23)_{12}=
     \sqrt{\frac{2}{3}}\left(\sqrt{\frac{1}{2}}\right)+\left(-\sqrt{\frac{1}{6}}\right)\left(0\right)+\left(-\sqrt{\frac{1}{6}}\right)\left(-\sqrt{\frac{1}{2}}\right)=\frac{\sqrt{3}}{2}\\
     D^{[1]}(23)_{21}=\frac{\sqrt{3}}{2} ,  D^{[1]}(23)_{22}=\frac{1}{2}
    \end{gathered}
\end{equation}
Obtaining
\begin{equation}
    D^{[1]}(23)=\left( \begin{array}{cc}
       - \frac{1}{2}  & \frac{\sqrt{3}}{2} \\
         \frac{\sqrt{3}}{2} & \frac{1}{2}
     \end{array}\right)
\end{equation}
The same irrep obtained by Young-Yamanouchi algorithm in Eq(\ref{eq:irep2321}). Note how this procedure allows one to compute any matrix element for any permutation, not only adjacent transpositions. In a general case this can be written as
\begin{equation}
    D^{[\lambda]}(\pi)_{Y_i,Y_j}= \sum_{s\in \omega}    \bra{\lambda,\omega,Y_i} \ket{s} \bra{\pi s}  \ket{\lambda,\omega,Y_j} \quad , \quad \forall \omega \in \lambda
    \label{eq:myirreps}
\end{equation}
In \nameref{AppendixI} we show how this construction facilitates the computation of elements in the Schur transform for certain kind of quantum systems.
