# Supplementary material for: Kronecker states: a powerful source of multipartite maximally entangled states in quantum information
Source: arXiv:2504.16256 source file (2025-04-22)
Supplement: Supplementary file 2 [file Appendix02.tex]

\label{AppendixII}
In the \nameref{Invariants} section we discussed about the freedom to choose invariants as basis for the invariant ring, in this appendix we explore the different invariants that can be obtained for the four qubits case and their correspondence with the $B,L,M$ and $D_{xy}$ invariants. 
\begin{equation}
F_0:=
\begin{tikzpicture}[basel={-.5}]
\draw[fill=white, postaction={pattern =crosshatch}] (0,0) circle[radius=0.2];
\draw[fill=white, postaction={pattern =crosshatch}] (2, 0) circle[radius=0.2];
\draw[fill=white, postaction={pattern =crosshatch}] (4, 0) circle[radius=0.2];
\draw[fill=white, postaction={pattern =crosshatch}] (4,2) circle[radius=0.2]; 
\draw[fill=white, postaction={pattern =crosshatch}] (2,2) circle[radius=0.2];
\draw[fill=white, postaction={pattern =crosshatch}] (0,2) circle[radius=0.2];
\draw[markxo={0.5}{0.6}] (0,0.1) to (2,0.1);
\draw[markxo={0.5}{0.6}] (0,-0.1) to (2,-0.1);
\draw[markxo={0.5}{0.6}] (2,0.1) to (4,0.1);
\draw[markxo={0.5}{0.6}] (2,-0.1) to (4,-0.1);
\draw[markxo={0.5}{0.6}] (3.9,0) to (3.9,2);
\draw[markxo={0.5}{0.6}] (4.1,0) to (4.1,2);
\draw[markxo={0.5}{0.6}] (-0.1,0) to (-0.1,2);
\draw[markxo={0.5}{0.6}] (0.1,0) to (0.1,2);
\draw[markxo={0.5}{0.6}] (0,2.1) to (2,2.1);
\draw[markxo={0.5}{0.6}] (0,1.9) to (2,1.9);
\draw[markxo={0.5}{0.6}] (2,2.1) to (4,2.1);
\draw[markxo={0.5}{0.6}] (2,1.9) to (4,1.9);
\end{tikzpicture} \equiv 2B^3-12D_{xy}-6LB-12MB.
\end{equation}
